# Supplementary material for: Backdoor Graph Condensation
Source: arXiv:2407.11025 source file (2025-03-31)
Supplement: Supplementary file 1 [file main-appendix.tex]

% \begin{table*}
% \caption{Varying the poison ratio.}
% \label{tab:cross}
% \vspace{-2mm}
% \subfloat[Cora]{%\scriptsize
% % \setlength{\tabcolsep}{1.8pt}
% \input{sections/experiment-results/poison-ratio/cora}
% }%\quad 
% \\
% % \newline
% % \newline\noindent
% \subfloat[Citeseer]{%\scriptsize
% % \setlength{\tabcolsep}{1.8pt}
% \begin{tabular}{c}
% \input{sections/experiment-results/poison-ratio/citeseer}
% \end{tabular}
% }
% \end{table*}
\begin{table*}
\centering
\vskip -0.13in
\caption{Varying the poisoning ratio.}
\vskip -0.1in
\label{tab:poisoning-ratio-appendix}
\begin{threeparttable}
\scalebox{0.88}{
\begin{tabular}{c|c|c|cc|cc|cc}
\hline
\multirow{2}{*}{Datasets} &
  \multirow{2}{*}{Poison Rate} &
  \multirow{2}{*}{Ratio (r)} &
  \multicolumn{2}{c|}{DC-Graph} &
  \multicolumn{2}{c|}{GCond} &
  \multicolumn{2}{c}{GCond-X} \\ \cline{4-9} 
                           &                       &        & CTA     & ASR     & CTA     & ASR     & CTA     & ASR     \\ \hline
% \multirow{12}{*}{Cora}     & \multirow{3}{*}{0.05} & 1.30\% & 75.60 (1.24) & 100.0 (0.00)   & 80.57 (0.17) & 100.0 (0.00)   & 76.13 (0.95) & 100.0 (0.00)   \\
%                            &                       & 2.60\% & 76.10 (0.36) & 100.0 (0.00)   & 79.87 (0.78) & 100.0 (0.00)   & 78.50 (1.14) & 100.0 (0.00)   \\
%                            &                       & 5.20\% & 77.13 (0.54) & 100.0 (0.00)   & 80.13 (0.48) & 100.0 (0.00)   & 79.57 (0.58) & 100.0 (0.00)   \\ \cline{2-9} 
\multirow{9}{*}{Cora}     & \multirow{3}{*}{0.10}  & 1.30\% & 75.90 (0.34) & 100.0 (0.00)   & 81.23 (0.41) & 100.0 (0.00)   & 76.30 (1.08) & 100.0 (0.00)   \\
                           &                       & 2.60\% & 75.59 (0.63) & 100.0 (0.00)   & 80.67 (0.69) & 100.0 (0.00)   & 79.77 (0.57) & 100.0 (0.00)   \\
                           &                       & 5.20\% & 78.43 (0.35) & 100.0 (0.00)   & 80.70 (0.28) & 100.0 (0.00)   & 81.17 (0.90) & 100.0 (0.00)   \\ \cline{2-9} 
                           & \multirow{3}{*}{0.15} & 1.30\% & 75.26 (0.94) & 100.0 (0.00)   & 80.06 (0.24) & 100.0 (0.00)   & 75.30 (1.35) & 100.0 (0.00)   \\
                           &                       & 2.60\% & 75.00 (0.51) & 100.0 (0.00)   & 80.00 (0.52) & 100.0 (0.00)   & 78.10 (0.71) & 100.0 (0.00)   \\
                           &                       & 5.20\% & 77.47 (0.31) & 100.0 (0.00)   & 79.63 (0.50) & 100.0 (0.00)   & 79.40 (0.36) & 100.0 (0.00)   \\ \cline{2-9} 
                           & \multirow{3}{*}{0.20}  & 1.30\% & 75.13 (0.53) & 99.93 (0.05) & 78.33 (0.89) & 100.0 (0.00)   & 75.07 (0.37) & 100.0 (0.00)   \\
                           &                       & 2.60\% & 73.83 (0.34) & 100.0 (0.00)   & 79.51 (0.57) & 100.0 (0.00)   & 72.33 (0.93) & 100.0 (0.00)   \\
                           &                       & 5.20\% & 76.00 (0.73) & 100.0 (0.00)   & 78.63 (0.21) & 100.0 (0.00)   & 76.83 (0.68) & 100.0 (0.00)   \\ \hline
% \multirow{12}{*}{Citeseer} & \multirow{3}{*}{0.05} & 0.90\% & 70.30 (0.24) & 100.0 (0.00)   & 67.40 (0.43) & 100.0 (0.00)   & 72.06 (0.02) & 100.0 (0.00)   \\
%                            &                       & 1.80\% & 69.47 (1.01) & 100.0 (0.00)   & 69.27 (0.05) & 100.0 (0.00)   & 71.20 (0.57) & 100.0 (0.00)   \\
%                            &                       & 3.60\% & 69.20 (0.28) & 100.0 (0.00)   & 67.47 (0.71) & 100.0 (0.00)   & 72.23 (3.93) & 100.0 (0.00)   \\ \cline{2-9} 
\multirow{9}{*}{Citeseer}  & \multirow{3}{*}{0.10}  & 0.90\% & 70.27 (0.24) & 100.0 (0.00)   & 67.98 (0.94) & 100.0 (0.00)   & 65.07 (0.39) & 100.0 (0.00)   \\
                           &                       & 1.80\% & 68.17 (0.83) & 100.0 (0.00)   & 65.57 (0.87) & 100.0 (0.00)   & 67.13 (0.93) & 100.0 (0.00)   \\
                           &                       & 3.60\% & 68.83 (0.76) & 100.0 (0.00)   & 69.03 (1.08) & 100.0 (0.00)   & 67.27 (0.38) & 99.30 (0.57) \\ \cline{2-9} 
                           & \multirow{3}{*}{0.15} & 0.90\% & 69.20 (0.50) & 100.0 (0.00)   & 71.57 (1.32) & 100.0 (0.00)   & 73.03 (0.50) & 100.0 (0.00)   \\
                           &                       & 1.80\% & 69.37 (0.94) & 100.0 (0.00)   & 71.03 (0.09) & 100.0 (0.00)   & 72.40 (0.57)  & 100.0 (0.00)   \\
                           &                       & 3.60\% & 70.00 (0.22) & 100.0 (0.00)   & 70.60 (0.51) & 100.0 (0.00)   & 72.13 (0.83) & 100.0 (0.00)   \\ \cline{2-9} 
                           & \multirow{3}{*}{0.20}  & 0.90\% & 69.07 (0.33) & 100.0 (0.00)   & 67.77 (0.25) & 100.0 (0.00)   & 63.86 (1.04) & 100.0 (0.00)   \\
                           &                       & 1.80\% & 67.03 (0.99) & 100.0 (0.00)   & 69.43 (0.31) & 100.0 (0.00)   & 71.53 (0.70) & 100.0 (0.00)   \\
                           &                       & 3.60\% & 66.40 (0.39) & 100.0 (0.00)   & 69.27 (1.16) & 100.0 (0.00)   & 70.83 (0.57) & 99.40 (0.25) \\ \hline\hline
\multirow{2}{*}{Datasets} &
  \multirow{2}{*}{Poison Num} &
  \multirow{2}{*}{Ratio (r)} &
  \multicolumn{2}{c|}{DC-Graph} &
  \multicolumn{2}{c|}{GCond} &
  \multicolumn{2}{c}{GCond-X} \\ \cline{4-9}
                           &                       &        & CTA     & ASR     & CTA     & ASR     & CTA     & ASR     \\ \hline
% \multirow{12}{*}{Flickr}   & \multirow{3}{*}{40}   & 0.10\% & 45.96 (0.01) & 92.98 (0.01) & 46.66 (0.10) & 95.79 (1.44) & 46.24 (0.03) & 98.40 (0.04) \\
%                            &                       & 0.50\% & 46.59 (0.40) & 98.08 (1.46) & 47.14 (0.20) & 99.58 (0.24) & 46.20 (0.31) & 98.10 (0.03) \\
%                            &                       & 1.00\%    & 46.95 (0.21) & 95.55 (1.57) & 46.86 (0.20) & 94.09 (0.46) & 45.62 (0.24) & 100.0 (0.00) \\ \cline{2-9} 
\multirow{9}{*}{Flickr}   & \multirow{3}{*}{60}   & 0.10\% & 45.86 (0.25) & 99.56 (0.33) & 45.38 (0.29) & 99.13 (0.47) & 44.85 (0.34) & 100.0 (0.00)   \\
                           &                       & 0.50\% & 46.54 (0.36) & 96.86 (2.43) & 46.53 (0.19) & 99.96 (0.03) & 45.60 (0.18) & 100.0 (0.00)   \\
                           &                       & 1.00\%    & 46.34 (0.44) & 95.13 (0.40) & 46.92 (0.15) & 97.55 (1.77) & 45.87 (0.16) & 100.0 (0.00)   \\ \cline{2-9} 
                           & \multirow{3}{*}{80}   & 0.10\% & 46.48 (0.21) & 99.98 (0.02) & 46.54 (0.08) & 99.83 (0.07) & 46.15 (0.47) & 98.26 (1.59) \\
                           &                       & 0.50\% & 46.44 (0.13) & 99.25 (0.65) & 47.15 (0.08) & 99.97 (0.02) & 45.21 (0.44) & 99.58 (0.35) \\
                           &                       & 1.00\%    & 46.77 (0.30) & 99.11 (0.40) & 46.84 (0.09) & 99.77 (0.06) & 45.62 (0.17) & 95.51 (1.69) \\ \cline{2-9} 
                           & \multirow{3}{*}{100}  & 0.10\% & 46.18 (0.03) & 100.0 (0.00)   & 46.18 (0.19) & 99.66 (0.12) & 46.19 (0.70) & 97.21 (2.24) \\
                           &                       & 0.50\% & 46.49 (0.34) & 99.05 (0.78) & 46.93 (0.17) & 98.46 (1.19) & 46.31 (0.31) & 100.0 (0.00)   \\
                           &                       & 1.00\%    & 46.76 (0.10) & 100.0 (0.00)   & 46.99 (0.04) & 99.17 (0.67) & 45.43 (0.59) & 100.0 (0.00)   \\ \hline
% \multirow{12}{*}{Reddit}   & \multirow{3}{*}{80}   & 0.05\% & 86.95 (0.30) & 90.12 (1.42) & 89.29 (0.07) & 93.81 (0.04) & 88.47 (0.42) & 90.89 (1.12) \\
%                            &                       & 0.10\% & 89.15 (0.12) & 88.26 (0.24) & 89.07 (0.22) & 90.35 (0.21) & 89.04 (0.01) & 94.78 (0.34) \\
%                            &                       & 0.20\% & 89.66 (0.13) & 89.01 (0.06) & 90.25 (1.43) & 94.06 (0.38) & 90.18 (0.11) & 92.60 (0.57) \\ \cline{2-9} 
\multirow{9}{*}{Reddit}       & \multirow{3}{*}{130}  & 0.05\% & 85.74 (0.86) & 96.12 (0.90) & 88.50 (0.10) & 97.14 (0.34) & 88.10 (0.28) & 96.15 (0.35) \\
                           &                       & 0.10\% & 89.18 (0.02) & 98.26 (1.06) & 90.37 (0.74) & 98.99 (0.19) & 90.29 (0.41) & 97.17 (0.42) \\
                           &                       & 0.20\% & 90.66 (0.53) & 97.81 (0.46) & 90.76 (0.14) & 98.39 (1.20) & 90.66 (1.27) & 96.44 (1.32) \\ \cline{2-9} 
                           & \multirow{3}{*}{180}  & 0.05\% & 85.40 (0.42) & 99.90 (0.03) & 88.37 (0.27) & 99.84 (0.14) & 88.04 (0.21) & 99.89 (0.05) \\
                           &                       & 0.10\% & 89.14 (0.05) & 99.93 (0.02) & 90.16 (0.22) & 99.99 (0.01) & 90.10 (0.51) & 99.78 (0.13) \\
                           &                       & 0.20\% & 90.38 (0.42) & 99.90 (0.03) & 90.61 (0.41) & 99.06 (0.91) & 90.15 (0.21) & 97.60 (1.42) \\ \cline{2-9} 
                           & \multirow{3}{*}{230}  & 0.05\% & 85.38 (0.28) & 98.29 (0.17) & 88.14 (0.16) & 98.92 (0.73) & 87.47 (0.42) & 99.10 (0.44) \\
                           &                       & 0.10\% & 89.01 (0.04) & 99.44 (0.21) & 89.93 (0.83) & 99.03 (0.18) & 89.14 (0.26) & 99.27 (0.14) \\
                           &                       & 0.20\% & 89.94 (0.76) & 99.08 (0.05) & 90.40 (0.27) & 99.22 (0.42) & 90.09 (0.45) & 98.00 (0.37) \\ \hline
\end{tabular}
}
\begin{tablenotes}
    \item 
\end{tablenotes}
\end{threeparttable}
\vskip -0.05in
\end{table*}
