# Supplementary material for: Backdoor Graph Condensation
Source: arXiv:2407.11025 source file (2025-03-31)
Supplement: Supplementary file 3 [file main-appendix.tex]

\begin{table*}[h]
\centering
\vskip -0.13in
\caption{Attack performance comparison.}
\vskip -0.14in
\label{tab:main-performance-compare-appendxi}
\scalebox{0.9}{
\begin{tabular}{c|c|c|cc|cc|cc}
\hline
 &
   &
  {\color[HTML]{1F1F1F} } &
  \multicolumn{2}{c|}{GTA} &
  \multicolumn{2}{c|}{DOORPING} &
  \multicolumn{2}{c}{BGC} \\ \cline{4-9} 
\multirow{-2}{*}{\begin{tabular}{@{}c@{}} Cond. \\ Method \end{tabular}} &
  \multirow{-2}{*}{Datasets} &
  \multirow{-2}{*}{{\color[HTML]{1F1F1F} Ratio (r)}}&
  CTA &
  ASR &
  CTA &
  ASR &
  CTA &
  ASR \\ \hline
 &
   &
  {\color[HTML]{1F1F1F} 1.30\%} &
  68.97 (2.05) &
  100.0 (0.00) &
  66.10 (0.17) &
  100.0 (0.00) &
  \textbf{75.90 (0.94)} &
  \textbf{100.0 (0.00)} \\
 &
   &
  {\color[HTML]{1F1F1F} 2.60\%} &
  72.30 (0.75) &
  100.0 (0.00) &
  73.50 (0.96) &
  100.0 (0.00) &
  \textbf{75.00 (0.51)} &
  \textbf{100.0 (0.00)} \\
 &
  \multirow{-3}{*}{Cora} &
  {\color[HTML]{1F1F1F} 5.20\%} &
  75.93 (0.09) &
  100.0 (0.00) &
  76.00 (0.54) &
  100.0 (0.00) &
  \textbf{78.43 (0.31)} &
  \textbf{100.0 (0.00)} \\ \cline{2-9} 
 &
   &
  {\color[HTML]{1F1F1F} 0.90\%} &
  65.90 (1.02) &
  100.0 (0.00) &
  66.90 (1.07) &
  100.0 (0.00) &
  \textbf{70.27 (0.50)} &
  \textbf{100.0 (0.00)} \\
 &
   &
  {\color[HTML]{1F1F1F} 1.80\%} &
  67.43 (0.87) &
  100.0 (0.00) &
  67.20 (0.57) &
  100.0 (0.00) &
  \textbf{69.37 (0.94)} &
  \textbf{100.0 (0.00)} \\
 &
  \multirow{-3}{*}{Citeseer} &
  {\color[HTML]{1F1F1F} 3.60\%} &
  67.03 (1.00) &
  100.0 (0.00) &
  67.50 (0.36) &
  100.0 (0.00) &
  \textbf{70.00 (0.22)} &
  \textbf{100.0 (0.00)} \\ \cline{2-9} 
 &
   &
  {\color[HTML]{1F1F1F} 0.10\%} &
  45.09 (0.42) &
  90.13 (0.57) &
  45.20 (0.23) &
  91.05 (1.10) &
  \textbf{46.48 (0.21)} &
  \textbf{99.98 (0.02)} \\
 &
   &
  {\color[HTML]{1F1F1F} 0.50\%} &
  46.01 (0.05) &
  89.83 (0.78) &
  46.17 (0.11) &
  93.09 (2.35) &
  \textbf{46.44 (0.13)} &
  \textbf{99.25 (0.71)} \\
 &
  \multirow{-3}{*}{Flickr} &
  {\color[HTML]{1F1F1F} 1.00\%} &
  46.15 (0.12) &
  90.45 (0.44) &
  46.07 (0.07) &
  91.66 (0.83) &
  \textbf{46.77 (0.30)} &
  \textbf{99.11 (0.40)} \\ \cline{2-9} 
 &
   &
  {\color[HTML]{1F1F1F} 0.05\%} &
  85.75 (0.58) &
  90.32 (0.12) &
  85.07 (0.30) &
  94.17 (1.62) &
  \textbf{85.38 (0.42)} &
  \textbf{99.90 (0.03)} \\
 &
   &
  {\color[HTML]{1F1F1F} 0.10\%} &
  88.87 (0.24) &
  89.09 (0.94) &
  88.46 (0.21) &
  90.01 (0.70) &
  \textbf{89.14 (0.05)} &
  \textbf{99.93 (0.02)} \\
\multirow{-12}{*}{DC-Graph} &
  \multirow{-3}{*}{Reddit} &
  {\color[HTML]{1F1F1F} 0.20\%} &
  90.07 (0.32) &
  89.62 (0.34) &
  90.24 (0.14) &
  91.21 (0.93) &
  \textbf{90.38 (0.42)} &
  \textbf{99.90 (0.03)} \\ \hline\hline
 &
   &
  {\color[HTML]{1F1F1F} 1.30\%} &
  80.13 (0.56) &
  100.0 (0.00) &
  80.87 (0.73) &
  100.0 (0.00) &
  \textbf{81.23 (0.24)} &
  \textbf{100.0 (0.00)} \\
 &
   &
  {\color[HTML]{1F1F1F} 2.60\%} &
  79.93 (0.29) &
  100.0 (0.00) &
  79.77 (0.33) &
  100.0 (0.00) &
  \textbf{80.67 (0.52)} &
  \textbf{100.0 (0.00)} \\
 &
  \multirow{-3}{*}{Cora} &
  {\color[HTML]{1F1F1F} 5.20\%} &
  78.33 (0.71) &
  100.0 (0.00) &
  80.03 (0.42) &
  100.0 (0.00) &
  \textbf{80.70 (0.50)} &
  \textbf{100.0 (0.00)} \\ \cline{2-9} 
 &
   &
  {\color[HTML]{1F1F1F} 0.90\%} &
  69.30 (0.59) &
  100.0 (0.00) &
  54.60 (0.08) &
  100.0 (0.00) &
  \textbf{71.57 (1.32)} &
  \textbf{100.0 (0.00)} \\
 &
   &
  {\color[HTML]{1F1F1F} 1.80\%} &
  68.53 (0.29) &
  100.0 (0.00) &
  69.30 (0.80) &
  100.0 (0.00) &
  \textbf{71.03 (0.09)} &
  \textbf{100.0 (0.00)} \\
 &
  \multirow{-3}{*}{Citeseer} &
  {\color[HTML]{1F1F1F} 3.60\%} &
  69.07 (1.40) &
  100.0 (0.00) &
  68.03 (0.50) &
  100.0 (0.00) &
  \textbf{70.60 (0.51)} &
  \textbf{100.0 (0.00)} \\ \cline{2-9} 
 &
   &
  {\color[HTML]{1F1F1F} 0.10\%} &
  46.00 (0.07) &
  92.07 (0.19) &
  46.01 (0.16) &
  93.16 (0.03) &
  \textbf{46.54 (0.08)} &
  \textbf{99.83 (0.07)} \\
 &
   &
  {\color[HTML]{1F1F1F} 0.50\%} &
  46.32 (0.30) &
  96.53 (0.12) &
  46.50 (0.08) &
  95.33 (1.31) &
  \textbf{47.15 (0.08)} &
  \textbf{99.97 (0.02)} \\
 &
  \multirow{-3}{*}{Flickr} &
  {\color[HTML]{1F1F1F} 1.00\%} &
  45.82 (0.36) &
  94.57 (1.63) &
  45.69 (0.32) &
  93.54 (2.13) &
  \textbf{46.84 (0.09)} &
  \textbf{99.77 (0.06)} \\ \cline{2-9} 
 &
   &
  {\color[HTML]{1F1F1F} 0.05\%} &
  82.14 (0.26) &
  93.33 (2.61) &
  87.95 (0.39) &
  92.00 (2.08) &
  \textbf{88.50 (0.27)} &
  \textbf{99.84 (0.14)} \\
 &
   &
  {\color[HTML]{1F1F1F} 0.10\%} &
  83.10 (1.28) &
  96.25 (0.18) &
  89.71 (0.28) &
  98.33 (0.44) &
  \textbf{90.37 (0.22)} &
  \textbf{99.99 (0.01)} \\
\multirow{-12}{*}{GCond} &
  \multirow{-3}{*}{Reddit} &
  {\color[HTML]{1F1F1F} 0.20\%} &
  83.03 (0.53) &
  97.80 (0.22) &
  90.28 (0.30) &
  96.16 (3.18) &
  \textbf{90.40 (0.41)} &
  \textbf{99.06 (0.91)} \\ \hline\hline
 &
   &
  {\color[HTML]{1F1F1F} 1.30\%} &
  75.40 (1.85) &
  89.00 (0.08) &
  75.67 (0.74) &
  100.0 (0.00) &
  \textbf{76.30 (1.35)} &
  \textbf{100.0 (0.00)} \\
 &
   &
  {\color[HTML]{1F1F1F} 2.60\%} &
  79.27 (0.25) &
  88.57 (0.21) &
  79.63 (0.52) &
  100.0 (0.00) &
  \textbf{78.10 (0.71)} &
  \textbf{100.0 (0.00)} \\
 &
  \multirow{-3}{*}{Cora} &
  {\color[HTML]{1F1F1F} 5.20\%} &
  80.63 (0.82) &
  93.13 (0.05) &
  81.47 (0.25) &
  100.0 (0.00) &
  \textbf{79.40 (0.36)} &
  \textbf{100.0 (0.00)} \\ \cline{2-9} 
 &
   &
  {\color[HTML]{1F1F1F} 0.90\%} &
  69.00 (1.77) &
  89.47 (0.05) &
  55.47 (0.79) &
  92.00 (0.48) &
  \textbf{73.03 (0.50)} &
  \textbf{100.0 (0.00)} \\
 &
   &
  {\color[HTML]{1F1F1F} 1.80\%} &
  72.00 (0.22) &
  88.63 (0.26) &
  63.63 (0.49) &
  96.67 (0.62) &
  \textbf{72.40 (0.57)} &
  \textbf{100.0 (0.00)} \\
 &
  \multirow{-3}{*}{Citeseer} &
  {\color[HTML]{1F1F1F} 3.60\%} &
  69.23 (1.32) &
  85.13 (0.09) &
  55.47 (0.97) &
  90.55 (1.45) &
  \textbf{72.13 (0.83)} &
  \textbf{100.0 (0.00)} \\ \cline{2-9} 
 &
   &
  {\color[HTML]{1F1F1F} 0.10\%} &
  45.78 (0.22) &
  87.10 (0.33) &
  45.79 (0.05) &
  \textbf{100.0 (0.00)} &
  \textbf{46.15 (0.47)} &
  98.26 (1.19) \\
 &
   &
  {\color[HTML]{1F1F1F} 0.50\%} &
  45.21 (0.16) &
  83.44 (3.32) &
  45.09 (0.12) &
  \textbf{100.0 (0.00)} &
  \textbf{46.21 (0.44)} &
  99.58 (0.35) \\
 &
  \multirow{-3}{*}{Flickr} &
  {\color[HTML]{1F1F1F} 1.00\%} &
  45.11 (0.15) &
  81.29 (0.24) &
  45.12 (0.22) &
  \textbf{100.0 (0.00)} &
  \textbf{45.62 (0.17)} &
  95.51 (1.69) \\ \cline{2-9} 
 &
   &
  {\color[HTML]{1F1F1F} 0.05\%} &
  86.48 (0.43) &
  90.08 (1.20) &
  87.41 (0.63) &
  91.40 (1.98) &
  \textbf{87.47 (0.21)} &
  \textbf{99.79 (0.15)} \\
 &
   &
  {\color[HTML]{1F1F1F} 0.10\%} &
  87.34 (0.12) &
  95.23 (0.47) &
  88.44 (0.19) &
  92.81 (0.21) &
  \textbf{89.14 (0.51)} &
  \textbf{99.68 (0.30)} \\
\multirow{-12}{*}{GCond-X} &
  \multirow{-3}{*}{Reddit} &
  {\color[HTML]{1F1F1F} 0.20\%} &
  88.70 (0.22) &
  96.52 (0.13) &
  89.30 (0.23) &
  94.12 (0.43) &
  \textbf{90.09 (0.21)} &
  \textbf{97.60 (1.82)} \\ \hline\hline
 &
      &
  {\color[HTML]{1F1F1F} 1.30\%} &
  73.18 (2.03) &
  82.33 (1.34) &
  71.80 (14.21) &
  88.80 (0.90) &
  \textbf{79.73 (1.40)} &
  \textbf{98.30 (1.53)} \\
 &
   &
  {\color[HTML]{1F1F1F} 2.60\%} &
  77.66 (0.40) &
  85.22 (0.94) &
  79.30 (0.62) &
  87.50 (1.07) &
  \textbf{79.10 (1.04)} &
  \textbf{99.77 (0.15)} \\
 &
  \multirow{-3}{*}{Cora} &
  {\color[HTML]{1F1F1F} 5.20\%} &
  78.01 (0.16) &
  82.11 (0.14) &
  79.10 (0.63) &
  81.30 (1.27) &
  \textbf{79.67 (0.42)} &
  \textbf{98.13 (1.65)} \\ \cline{2-9} 
 &
   &
  {\color[HTML]{1F1F1F} 0.90\%} &
  59.02 (0.14) &
  85.46 (0.26) &
  58.57 (4.22) &
  86.80 (0.67) &
  \textbf{60.20 (3.64)} &
  \textbf{100.0 (0.00)} \\
 &
   &
  {\color[HTML]{1F1F1F} 1.80\%} &
  62.39 (1.33) &
  85.18 (0.91) &
  62.10 (1.05) &
  85.93 (1.31) &
  \textbf{63.03 (2.64)} &
  \textbf{100.0 (0.00)} \\
 &
  \multirow{-3}{*}{Citeseer} &
  {\color[HTML]{1F1F1F} 3.60\%} &
  61.99 (0.78) &
  86.54 (0.25) &
  62.40 (1.55) &
  87.33 (0.89) &
  \textbf{63.37 (2.06)} &
  \textbf{100.0 (0.00)} \\ \cline{2-9} 
 &
   &
  {\color[HTML]{1F1F1F} 0.10\%} &
  45.10 (0.67) &
  86.15 (1.23) &
  45.80 (0.13) &
  84.26 (0.24) &
  \textbf{46.32 (0.09)} &
  \textbf{99.98 (0.00)} \\
 &
   &
  {\color[HTML]{1F1F1F} 0.50\%} &
  45.79 (0.14) &
  86.38 (0.58) &
  46.02 (0.12) &
  85.59 (1.62) &
  \textbf{46.02 (0.21)} &
  \textbf{99.98 (0.00)} \\
 &
  \multirow{-3}{*}{Flickr} &
  {\color[HTML]{1F1F1F} 1.00\%} &
  45.19 (0.11) &
  86.35 (0.37) &
  45.99 (0.08) &
  85.46 (0.86) &
  \textbf{45.50 (0.06)} &
  \textbf{99.98 (0.00)} \\ \cline{2-9} 
 &
   &
  {\color[HTML]{1F1F1F} 0.05\%} &
  OOM &
  OOM &
  OOM &
  OOM &
  OOM &
  OOM \\
 &
   &
  {\color[HTML]{1F1F1F} 0.10\%} &
  OOM &
  OOM &
  OOM &
  OOM &
  OOM &
  OOM \\
\multirow{-12}{*}{GC-SNTK} &
  \multirow{-3}{*}{Reddit} &
  {\color[HTML]{1F1F1F} 0.20\%} &
  OOM &
  OOM &
  OOM &
  OOM &
  OOM &
  OOM \\ \hline
\end{tabular}
}
\vskip -0.1in
\end{table*}
