# Supplementary material for: Backdoor Graph Condensation
Source: arXiv:2407.11025 source file (2025-03-31)
Supplement: Supplementary file 4 [file performance-under-defence-appendix.tex]

% Please add the following required packages to your document preamble:
% \usepackage{multirow}
% \usepackage[table,xcdraw]{xcolor}
% Beamer presentation requires \usepackage{colortbl} instead of \usepackage[table,xcdraw]{xcolor}
\begin{table*}[]
\centering
\vskip -0.1in
\caption{Attack Performance against Defenses.}
\vskip -0.09in
\scalebox{0.9}{
\begin{threeparttable}

\begin{tabular}{c|c|c|cccc|cccc|cc}
\hline
 &
   &
   &
  \multicolumn{4}{c|}{Defensed-Prune} &
  \multicolumn{4}{c|}{Defensed-Randsmooth} &
  \multicolumn{2}{c}{Backdoor} \\ \cline{4-13} 
\multirow{-2}{*}{\begin{tabular}{@{}c@{}} Cond. \\ Method \end{tabular}} &
  \multirow{-2}{*}{Datasets} &
  \multirow{-2}{*}{Ratio (r)} &
  CTA &
  $\Delta$ CTA &
  ASR &
  $\Delta$ ASR &
  CTA &
  $\Delta$ CTA &
  ASR &
  $\Delta$ ASR &
  CTA &
  ASR \\ \hline
 &
   &
  1.30\% &
  67.43 &
  {\color[HTML]{8B7A70} -11.16\%} &
  96.10 &
  {\color[HTML]{8B7A70} -3.90\%} &
  67.76 &
  {\color[HTML]{8B7A70} -10.72\%} &
  98.80 &
  {\color[HTML]{8B7A70} -1.20\%} &
  75.90 &
  100.0 \\
 &
   &
  2.60\% &
  73.07 &
  {\color[HTML]{8B7A70} -2.57\%} &
  97.43 &
  {\color[HTML]{8B7A70} -2.57\%} &
  73.07 &
  {\color[HTML]{8B7A70} -2.57\%} &
  98.87 &
  {\color[HTML]{8B7A70} -1.13\%} &
  75.00 &
  100.0 \\
 &
  \multirow{-3}{*}{Cora} &
  5.20\% &
  75.67 &
  {\color[HTML]{8B7A70} -3.52\%} &
  98.86 &
  {\color[HTML]{8B7A70} -1.14\%} &
  75.67 &
  {\color[HTML]{8B7A70} -3.52\%} &
  98.87 &
  {\color[HTML]{8B7A70} -1.13\%} &
  78.43 &
  100.0 \\ \cline{2-13} 
 &
   &
  0.90\% &
  66.00 &
  {\color[HTML]{8B7A70} -6.08\%} &
  71.00 &
  {\color[HTML]{8B7A70} -29.00\%} &
  67.40 &
  {\color[HTML]{8B7A70} -4.08\%} &
  98.70 &
  {\color[HTML]{8B7A70} -1.30\%} &
  70.27 &
  100.0 \\
 &
   &
  1.80\% &
  67.80 &
  {\color[HTML]{8B7A70} -2.26\%} &
  67.97 &
  {\color[HTML]{8B7A70} -32.03\%} &
  67.77 &
  {\color[HTML]{8B7A70} -2.31\%} &
  98.77 &
  {\color[HTML]{8B7A70} -1.23\%} &
  69.37 &
  100.0 \\
 &
  \multirow{-3}{*}{Citeseer} &
  3.60\% &
  66.17 &
  {\color[HTML]{8B7A70} -5.47\%} &
  87.20 &
  {\color[HTML]{8B7A70} -12.80\%} &
  66.17 &
  {\color[HTML]{8B7A70} -5.47\%} &
  98.80 &
  {\color[HTML]{8B7A70} -1.20\%} &
  70.00 &
  100.0 \\ \cline{2-13} 
 &
   &
  0.10\% &
  46.30 &
  {\color[HTML]{8B7A70} -0.39\%} &
  97.85 &
  {\color[HTML]{8B7A70} -2.13\%} &
  46.03 &
  {\color[HTML]{8B7A70} -0.97\%} &
  99.98 &
  {\color[HTML]{8B7A70} 0.00\%} &
  46.48 &
  99.98 \\
 &
   &
  0.50\% &
  45.44 &
  {\color[HTML]{8B7A70} -2.15\%} &
  90.74 &
  {\color[HTML]{8B7A70} -8.57\%} &
  46.39 &
  {\color[HTML]{8B7A70} -0.11\%} &
  98.56 &
  {\color[HTML]{8B7A70} -0.70\%} &
  46.44 &
  99.25 \\
 &
  \multirow{-3}{*}{Flickr} &
  1.00\% &
  46.07 &
  {\color[HTML]{8B7A70} -1.50\%} &
  92.17 &
  {\color[HTML]{8B7A70} -7.00\%} &
  46.47 &
  {\color[HTML]{8B7A70} -0.64\%} &
  99.34 &
  {\color[HTML]{8B7A70} 0.23\%} &
  46.77 &
  99.11 \\ \cline{2-13} 
 &
   &
  0.05\% &
  84.95 &
  {\color[HTML]{8B7A70} -0.50\%} &
  92.70 &
  {\color[HTML]{8B7A70} -7.21\%} &
  85.20 &
  {\color[HTML]{8B7A70} -0.21\%} &
  99.92 &
  {\color[HTML]{8B7A70} 0.02\%} &
  85.38 &
  99.9 \\
 &
   &
  0.10\% &
  88.74 &
  {\color[HTML]{8B7A70} -0.45\%} &
  93.39 &
  {\color[HTML]{8B7A70} -6.54\%} &
  88.48 &
  {\color[HTML]{8B7A70} -0.74\%} &
  99.76 &
  {\color[HTML]{8B7A70} -0.17\%} &
  89.14 &
  99.93 \\
\multirow{-12}{*}{DC-Graph} &
  \multirow{-3}{*}{Reddit} &
  0.20\% &
  89.54 &
  {\color[HTML]{8B7A70} -0.93\%} &
  91.74 &
  {\color[HTML]{8B7A70} -8.17\%} &
  90.58 &
  {\color[HTML]{8B7A70} 0.22\%} &
  99.31 &
  {\color[HTML]{8B7A70} -0.59\%} &
  90.38 &
  99.90 \\ \hline\hline
 &
   &
  1.30\% &
  45.40 &
  {\color[HTML]{8B7A70} -44.11\%} &
  75.60 &
  {\color[HTML]{8B7A70} -24.40\%} &
  78.70 &
  {\color[HTML]{8B7A70} -3.11\%} &
  99.07 &
  {\color[HTML]{8B7A70} -0.93\%} &
  81.23 &
  100.0 \\
 &
   &
  2.60\% &
  54.67 &
  {\color[HTML]{8B7A70} -32.23\%} &
  65.10 &
  {\color[HTML]{8B7A70} -34.90\%} &
  78.67 &
  {\color[HTML]{8B7A70} -2.48\%} &
  99.10 &
  {\color[HTML]{8B7A70} -0.90\%} &
  80.67 &
  100.0 \\
 &
  \multirow{-3}{*}{Cora} &
  5.20\% &
  55.97 &
  {\color[HTML]{8B7A70} -30.64\%} &
  99.00 &
  {\color[HTML]{8B7A70} -1.00\%} &
  80.10 &
  {\color[HTML]{8B7A70} -0.74\%} &
  98.83 &
  {\color[HTML]{8B7A70} -1.17\%} &
  80.70 &
  100.0 \\ \cline{2-13} 
 &
   &
  0.90\% &
  36.17 &
  {\color[HTML]{8B7A70} -49.46\%} &
  95.10 &
  {\color[HTML]{8B7A70} -4.90\%} &
  68.86 &
  {\color[HTML]{8B7A70} -3.79\%} &
  99.30 &
  {\color[HTML]{8B7A70} -0.70\%} &
  71.57 &
  100.0 \\
 &
   &
  1.80\% &
  48.87 &
  {\color[HTML]{8B7A70} -31.20\%} &
  85.70 &
  {\color[HTML]{8B7A70} -14.30\%} &
  62.90 &
  {\color[HTML]{8B7A70} -11.45\%} &
  99.37 &
  {\color[HTML]{8B7A70} -0.63\%} &
  71.03 &
  100.0 \\
 &
  \multirow{-3}{*}{Citeseer} &
  3.60\% &
  40.43 &
  {\color[HTML]{8B7A70} -42.73\%} &
  71.70 &
  {\color[HTML]{8B7A70} -28.30\%} &
  60.80 &
  {\color[HTML]{8B7A70} -13.88\%} &
  98.70 &
  {\color[HTML]{8B7A70} -1.30\%} &
  70.60 &
  100.0 \\ \cline{2-13} 
 &
   &
  0.10\% &
  41.52 &
  {\color[HTML]{8B7A70} -10.79\%} &
  90.03 &
  {\color[HTML]{8B7A70} -9.82\%} &
  45.57 &
  {\color[HTML]{8B7A70} -2.08\%} &
  97.53 &
  {\color[HTML]{8B7A70} -2.30\%} &
  46.54 &
  99.83 \\
 &
   &
  0.50\% &
  40.91 &
  {\color[HTML]{8B7A70} -13.23\%} &
  89.24 &
  {\color[HTML]{8B7A70} -10.73\%} &
  45.12 &
  {\color[HTML]{8B7A70} -4.31\%} &
  88.04 &
  {\color[HTML]{8B7A70} -11.93\%} &
  47.15 &
  99.97 \\
 &
  \multirow{-3}{*}{Flickr} &
  1.00\% &
  42.31 &
  {\color[HTML]{8B7A70} -9.67\%} &
  88.33 &
  {\color[HTML]{8B7A70} -11.47\%} &
  45.93 &
  {\color[HTML]{8B7A70} -1.94\%} &
  94.22 &
  {\color[HTML]{8B7A70} -5.56\%} &
  46.84 &
  99.77 \\ \cline{2-13} 
 &
   &
  0.05\% &
  67.14 &
  {\color[HTML]{8B7A70} -24.14\%} &
  91.28 &
  {\color[HTML]{8B7A70} -8.57\%} &
  72.99 &
  {\color[HTML]{8B7A70} -17.53\%} &
  99.97 &
  {\color[HTML]{8B7A70} 0.13\%} &
  88.5 &
  99.84 \\
 &
   &
  0.10\% &
  40.49 &
  {\color[HTML]{8B7A70} -55.20\%} &
  87.86 &
  {\color[HTML]{8B7A70} -12.13\%} &
  87.14 &
  {\color[HTML]{8B7A70} -3.57\%} &
  99.95 &
  {\color[HTML]{8B7A70} -0.04\%} &
  90.37 &
  99.99 \\
\multirow{-12}{*}{GCond} &
  \multirow{-3}{*}{Reddit} &
  0.20\% &
  56.74 &
  {\color[HTML]{8B7A70} -37.23\%} &
  88.15 &
  {\color[HTML]{8B7A70} -11.01\%} &
  87.01 &
  {\color[HTML]{8B7A70} -3.75\%} &
  95.73 &
  {\color[HTML]{8B7A70} -3.36\%} &
  90.40 &
  99.06 \\ \hline\hline
 &
   &
  1.30\% &
  72.03 &
  {\color[HTML]{8B7A70} -5.60\%} &
  73.67 &
  {\color[HTML]{8B7A70} -26.33\%} &
  75.70 &
  {\color[HTML]{8B7A70} -0.79\%} &
  98.87 &
  {\color[HTML]{8B7A70} -1.13\%} &
  76.30 &
  100.0 \\
 &
   &
  2.60\% &
  71.63 &
  {\color[HTML]{8B7A70} -8.28\%} &
  67.73 &
  {\color[HTML]{8B7A70} -32.27\%} &
  75.47 &
  {\color[HTML]{8B7A70} -3.37\%} &
  98.87 &
  {\color[HTML]{8B7A70} -1.13\%} &
  78.10 &
  100.0 \\
 &
  \multirow{-3}{*}{Cora} &
  5.20\% &
  77.53 &
  {\color[HTML]{8B7A70} -2.36\%} &
  89.80 &
  {\color[HTML]{8B7A70} -10.20\%} &
  76.93 &
  {\color[HTML]{8B7A70} -3.11\%} &
  98.90 &
  {\color[HTML]{8B7A70} -1.10\%} &
  79.40 &
  100.0 \\ \cline{2-13} 
 &
   &
  0.90\% &
  56.13 &
  {\color[HTML]{8B7A70} -23.14\%} &
  81.39 &
  {\color[HTML]{8B7A70} -18.61\%} &
  56.60 &
  {\color[HTML]{8B7A70} -22.50\%} &
  88.24 &
  {\color[HTML]{8B7A70} -11.76\%} &
  73.03 &
  100.0 \\
 &
   &
  1.80\% &
  65.37 &
  {\color[HTML]{8B7A70} -9.71\%} &
  80.10 &
  {\color[HTML]{8B7A70} -19.90\%} &
  55.43 &
  {\color[HTML]{8B7A70} -23.44\%} &
  88.70 &
  {\color[HTML]{8B7A70} -11.30\%} &
  72.40 &
  100.0 \\
 &
  \multirow{-3}{*}{Citeseer} &
  3.60\% &
  60.10 &
  {\color[HTML]{8B7A70} -16.68\%} &
  87.20 &
  {\color[HTML]{8B7A70} -12.80\%} &
  55.10 &
  {\color[HTML]{8B7A70} -23.61\%} &
  81.38 &
  {\color[HTML]{8B7A70} -18.62\%} &
  72.13 &
  100.0 \\ \cline{2-13} 
 &
   &
  0.10\% &
  42.14 &
  {\color[HTML]{8B7A70} -8.69\%} &
  65.93 &
  {\color[HTML]{8B7A70} -32.90\%} &
  45.02 &
  {\color[HTML]{8B7A70} -2.45\%} &
  99.97 &
  {\color[HTML]{8B7A70} 1.74\%} &
  46.15 &
  98.26 \\
 &
   &
  0.50\% &
  43.99 &
  {\color[HTML]{8B7A70} -2.70\%} &
  70.06 &
  {\color[HTML]{8B7A70} -29.64\%} &
  45.83 &
  {\color[HTML]{8B7A70} 1.37\%} &
  93.65 &
  {\color[HTML]{8B7A70} -5.96\%} &
  45.21 &
  99.58 \\
 &
  \multirow{-3}{*}{Flickr} &
  1.00\% &
  45.11 &
  {\color[HTML]{8B7A70} -1.12\%} &
  80.07 &
  {\color[HTML]{8B7A70} -16.17\%} &
  45.21 &
  {\color[HTML]{8B7A70} -0.90\%} &
  98.29 &
  {\color[HTML]{8B7A70} 2.91\%} &
  45.62 &
  95.51 \\ \cline{2-13} 
 &
   &
  0.05\% &
  87.12 &
  {\color[HTML]{8B7A70} -0.40\%} &
  90.15 &
  {\color[HTML]{8B7A70} -9.75\%} &
  88.26 &
  {\color[HTML]{8B7A70} 0.90\%} &
  98.87 &
  {\color[HTML]{8B7A70} -1.02\%} &
  87.47 &
  99.89 \\
 &
   &
  0.10\% &
  88.69 &
  {\color[HTML]{8B7A70} -0.50\%} &
  92.78 &
  {\color[HTML]{8B7A70} -7.02\%} &
  89.55 &
  {\color[HTML]{8B7A70} 0.46\%} &
  94.15 &
  {\color[HTML]{8B7A70} -5.64\%} &
  89.14 &
  99.78 \\
\multirow{-12}{*}{GCond-X} &
  \multirow{-3}{*}{Reddit} &
  0.20\% &
  89.80 &
  {\color[HTML]{8B7A70} -0.32\%} &
  91.72 &
  {\color[HTML]{8B7A70} -6.02\%} &
  89.90 &
  {\color[HTML]{8B7A70} -0.21\%} &
  98.64 &
  {\color[HTML]{8B7A70} 1.07\%} &
  90.09 &
  97.6 \\ \hline\hline
 &
   &
  1.30\% &
  74.80 &
  {\color[HTML]{8B7A70} -6.18\%} &
  84.13 &
  {\color[HTML]{8B7A70} -14.42\%} &
  -- &
  -- &
  -- &
  -- &
  79.73 &
  98.30 \\
 &
   &
  2.60\% &
  76.10 &
  {\color[HTML]{8B7A70} -3.79\%} &
  93.30 &
  {\color[HTML]{8B7A70} -6.48\%} &
  -- &
  -- &
  -- &
  -- &
  79.10 &
  99.77 \\
 &
  \multirow{-3}{*}{Cora} &
  5.20\% &
  77.67 &
  {\color[HTML]{8B7A70} -2.51\%} &
  85.30 &
  {\color[HTML]{8B7A70} -13.07\%} &
  -- &
  -- &
  -- &
  -- &
  79.67 &
  98.13 \\ \cline{2-13} 
 &
   &
  0.90\% &
  59.20 &
  {\color[HTML]{8B7A70} -1.66\%} &
  91.90 &
  {\color[HTML]{8B7A70} -8.10\%} &
  -- &
  -- &
  -- &
  -- &
  60.20 &
  100.0 \\
 &
   &
  1.80\% &
  61.13 &
  {\color[HTML]{8B7A70} -3.01\%} &
  94.13 &
  {\color[HTML]{8B7A70} -5.87\%} &
  -- &
  -- &
  -- &
  -- &
  63.03 &
  100.0 \\
 &
  \multirow{-3}{*}{Citeseer} &
  3.60\% &
  60.27 &
  {\color[HTML]{8B7A70} -4.89\%} &
  98.50 &
  {\color[HTML]{8B7A70} -1.50\%} &
  -- &
  -- &
  -- &
  -- &
  63.37 &
  100.0 \\ \cline{2-13} 
 &
   &
  0.10\% &
  45.45 &
  {\color[HTML]{8B7A70} -1.88\%} &
  90.77 &
  {\color[HTML]{8B7A70} -9.21\%} &
  -- &
  -- &
  -- &
  -- &
  46.32 &
  99.98 \\
 &
   &
  0.50\% &
  45.27 &
  {\color[HTML]{8B7A70} -1.63\%} &
  89.92 &
  {\color[HTML]{8B7A70} -10.06\%} &
  -- &
  -- &
  -- &
  -- &
  46.02 &
  99.98 \\
 &
  \multirow{-3}{*}{Flickr} &
  1.00\% &
  45.29 &
  {\color[HTML]{8B7A70} -0.46\%} &
  88.79 &
  {\color[HTML]{8B7A70} -11.19\%} &
  -- &
  -- &
  -- &
  -- &
  45.50 &
  99.98 \\ \cline{2-13} 
 &
   &
  0.05\% &
  OOM &
  -- &
  OOM &
  -- &
  OOM &
  -- &
  OOM &
  -- &
  OOM &
  OOM \\
 &
   &
  0.10\% &
  OOM &
  -- &
  OOM &
  -- &
  OOM &
  -- &
  OOM &
  -- &
  OOM &
  OOM \\
\multirow{-12}{*}{GC-SNTK} &
  \multirow{-3}{*}{Reddit} &
  0.20\% &
  OOM &
  -- &
  OOM &
  -- &
  OOM &
  -- &
  OOM &
  -- &
  OOM &
  OOM \\ \hline
\end{tabular}
\begin{tablenotes}
    % \item $\Delta$ CTA: the influence of defense on the clean test accuracy. \qquad\quad$\Delta$ ASR: the influence of defense on the attack success rate.%, representing the performance of models trained on backdoored graphs. 
    \item 
\end{tablenotes}
\end{threeparttable}
}
\label{tab:performance-under-defense-appendix}
% \vskip -0.07in
\end{table*}
